# Supplementary material for: Nonlinear corrections in the quantization of a weakly nonideal Bose gas at zero temperature
Source: arXiv:2103.12030 ancillary file (2022-06-13)
Supplement: Supplementary file 1 [file commutators_coefficients_v2.pdf]

→ /\* Definitions (197)-(200): \gamma\_{j}/\omega=J, \gamma\_{l}/\omega=L, \gamma\_{j+l}/\omega=S \*/;

(%i1) /\* M\_{j,l}^{\star}\omega\_{l}/c\_{j}=Mp1(J,L,S) \*/

Mp1(J,L,S):=((J+L+sqrt(S^2+1)-1)·(J+L-sqrt(J^2+1)-sqrt(L^2+1)+1)  
-(sqrt(J^2+1)-J)·(sqrt(L^2+1)-L))/(L·((J+L)^2-S^2));

$$(\%o1) \quad Mp1(J, L, S) := \frac{(J+L+\sqrt{S^2+1}-1)(J+L-\sqrt{J^2+1}-\sqrt{L^2+1}+1)+\left(-(\sqrt{J^2+1}-J)\right)(\sqrt{L^2+1}-L)}{L\left((J+L)^2-S^2\right)}$$

(%i2) /\* M\_{j,-j-1}^{\star}\omega\_{j+1}/c\_{j}=Mp2(J,L,S) \*/

Mp2(J,L,S):=((J+S+sqrt(L^2+1)-1)·(J+S-sqrt(J^2+1)-sqrt(S^2+1)+1)  
-(sqrt(J^2+1)-J)·(sqrt(S^2+1)-S))/(S·((J+S)^2-L^2));

$$(\%o2) \quad Mp2(J, L, S) := \frac{(J+S+\sqrt{L^2+1}-1)(J+S-\sqrt{J^2+1}-\sqrt{S^2+1}+1)+\left(-(\sqrt{J^2+1}-J)\right)(\sqrt{S^2+1}-S)}{S\left((J+S)^2-L^2\right)}$$

(%i3) /\* M\_{j,-l}^{\star}\omega\_{l}/c\_{j}=Mm1(J,L,S) \*/

Mm1(J,L,S):=((sqrt(S^2+1)+J-L-1)·((sqrt(J^2+1)-J-1)·(sqrt(L^2+1)-L)+1)  
+(sqrt(J^2+1)-J-sqrt(L^2+1)+L))/(L·((J-L)^2-S^2)·(sqrt(L^2+1)-L));

$$(\%o3) \quad Mm1(J, L, S) := \frac{(\sqrt{S^2+1}+J-L-1)\left((\sqrt{J^2+1}-J-1)(\sqrt{L^2+1}-L)+1\right)+(\sqrt{J^2+1}-J-\sqrt{L^2+1}+L)}{L\left((J-L)^2-S^2\right)(\sqrt{L^2+1}-L)}$$

(%i4) /\* M\_{j,j+1}^{\star}\omega\_{j+1}/c\_{j}=Mm2(J,L,S) \*/

Mm2(J,L,S):=((sqrt(L^2+1)+J-S-1)·((sqrt(J^2+1)-J-1)·(sqrt(S^2+1)-S)+1)  
+(sqrt(J^2+1)-J-sqrt(S^2+1)+S))/(S·((J-S)^2-L^2)·(sqrt(S^2+1)-S));

$$(\%o4) \quad Mm2(J, L, S) := \frac{(\sqrt{L^2+1}+J-S-1)\left((\sqrt{J^2+1}-J-1)(\sqrt{S^2+1}-S)+1\right)+(\sqrt{J^2+1}-J-\sqrt{S^2+1}+S)}{S\left((J-S)^2-L^2\right)(\sqrt{S^2+1}-S)}$$

```
(%i5) /* Definition (224): \gamma_{a}/\omega=A, \gamma_{b}/\omega=B, K_{a,b}^{+}\omega c_{b}/c_{a}=K(A,B) */
K(A,B):=(1/(sqrt(B^2+1)-B))\cdot(1-(sqrt(A^2+1)-A))-1
-(sqrt((A+B)^2+1)+A+B)\cdot((sqrt(A^2+1)-A)\cdot(1-1/(sqrt(B^2+1)-B))-1)/(2\cdot B\cdot(A+B));
```

```
(%o5) K(A,B):=
```

$$\frac{\frac{1}{\sqrt{B^2+1}-B} \left( 1 - (\sqrt{A^2+1}-A) \right) - 1 + \left( -\sqrt{(A+B)^2+1} + A + B \right) \left( (\sqrt{A^2+1}-A) \left( 1 - \frac{1}{\sqrt{B^2+1}-B} \right) - 1 \right)}{2 B (A+B)}$$

```
(%i6) /* Equality (201) */
ratsimp(Mp1(J,L,S)-Mp2(J,L,S)+Mm1(J,L,S)-Mm2(J,L,S));
```

```
(%o6) 0
```

```
(%i7) /* Equality (204) (see formulas (202), (203)) */
ratsimp(((J+L-sqrt(S^2+1))/(sqrt(L^2+1)-L))\cdot Mp1(J,L,S)-((J+S-sqrt(L^2+1))/(sqrt(S^2+1)-S))\cdot Mp2(J,L,S)
+((J-L-sqrt(S^2+1))/(sqrt(L^2+1)+L))\cdot Mm1(J,L,S)-((J-S-sqrt(L^2+1))/(sqrt(S^2+1)+S))\cdot Mm2(J,L,S));
```

```
(%o7) 0
```

```
(%i8) /* Equality (206) (see formula (205)) */
ratsimp(L\cdot Mp1(J,L,S)+(J+S)\cdot Mp2(J,L,S)-L\cdot Mm1(J,L,S)+(J-S)\cdot Mm2(J,L,S)-2);
```

```
(%o8) 0
```

```
(%i9) /* Equality (225) (see formula (223)) */
ratsimp(K(A,B)-(2\cdot(A+B)\cdot(2\cdot A+B-sqrt(B^2+1))/(sqrt((A+B)^2+1)-A-B))\cdot Mp2(A,B,A+B)
-(2\cdot B\cdot(sqrt(B^2+1)-B)/(sqrt((A+B)^2+1)-A-B))\cdot Mm1(A,B,A+B)
+2\cdot((A+B+1-sqrt(A^2+1)-sqrt(B^2+1))/(2\cdot B\cdot(sqrt((A+B)^2+1)-A-B)\cdot(sqrt(B^2+1)-B))-1));
```

```
(%o9) 0
```

```
(%i10) /* Equality (227) (see formula (226)) */
ratsimp(((sqrt((A+B)^2+1)-A-B)/(sqrt(B^2+1)+B))\cdot K(A,B)
+2\cdot(A+B)\cdot Mp2(A,B,A+B)-2\cdot B\cdot Mm1(A,B,A+B)-(sqrt(A^2+1)-A+sqrt(B^2+1)+B-1)/B);
```

```
(%o10) 0
```
